# Supplementary material for: iSeg: Interactive 3D Segmentation via Interactive Attention
Source: arXiv:2404.03219 source file (2024-10-28)
Supplement: Supplementary file 1 [file cross_png.tex]

\begin{figure}
\centering
\newcommand{\pl}{-3}
% trim: left, bottom, right, top
\begin{overpic}[width=\linewidth, trim=100 10 150 50, clip]{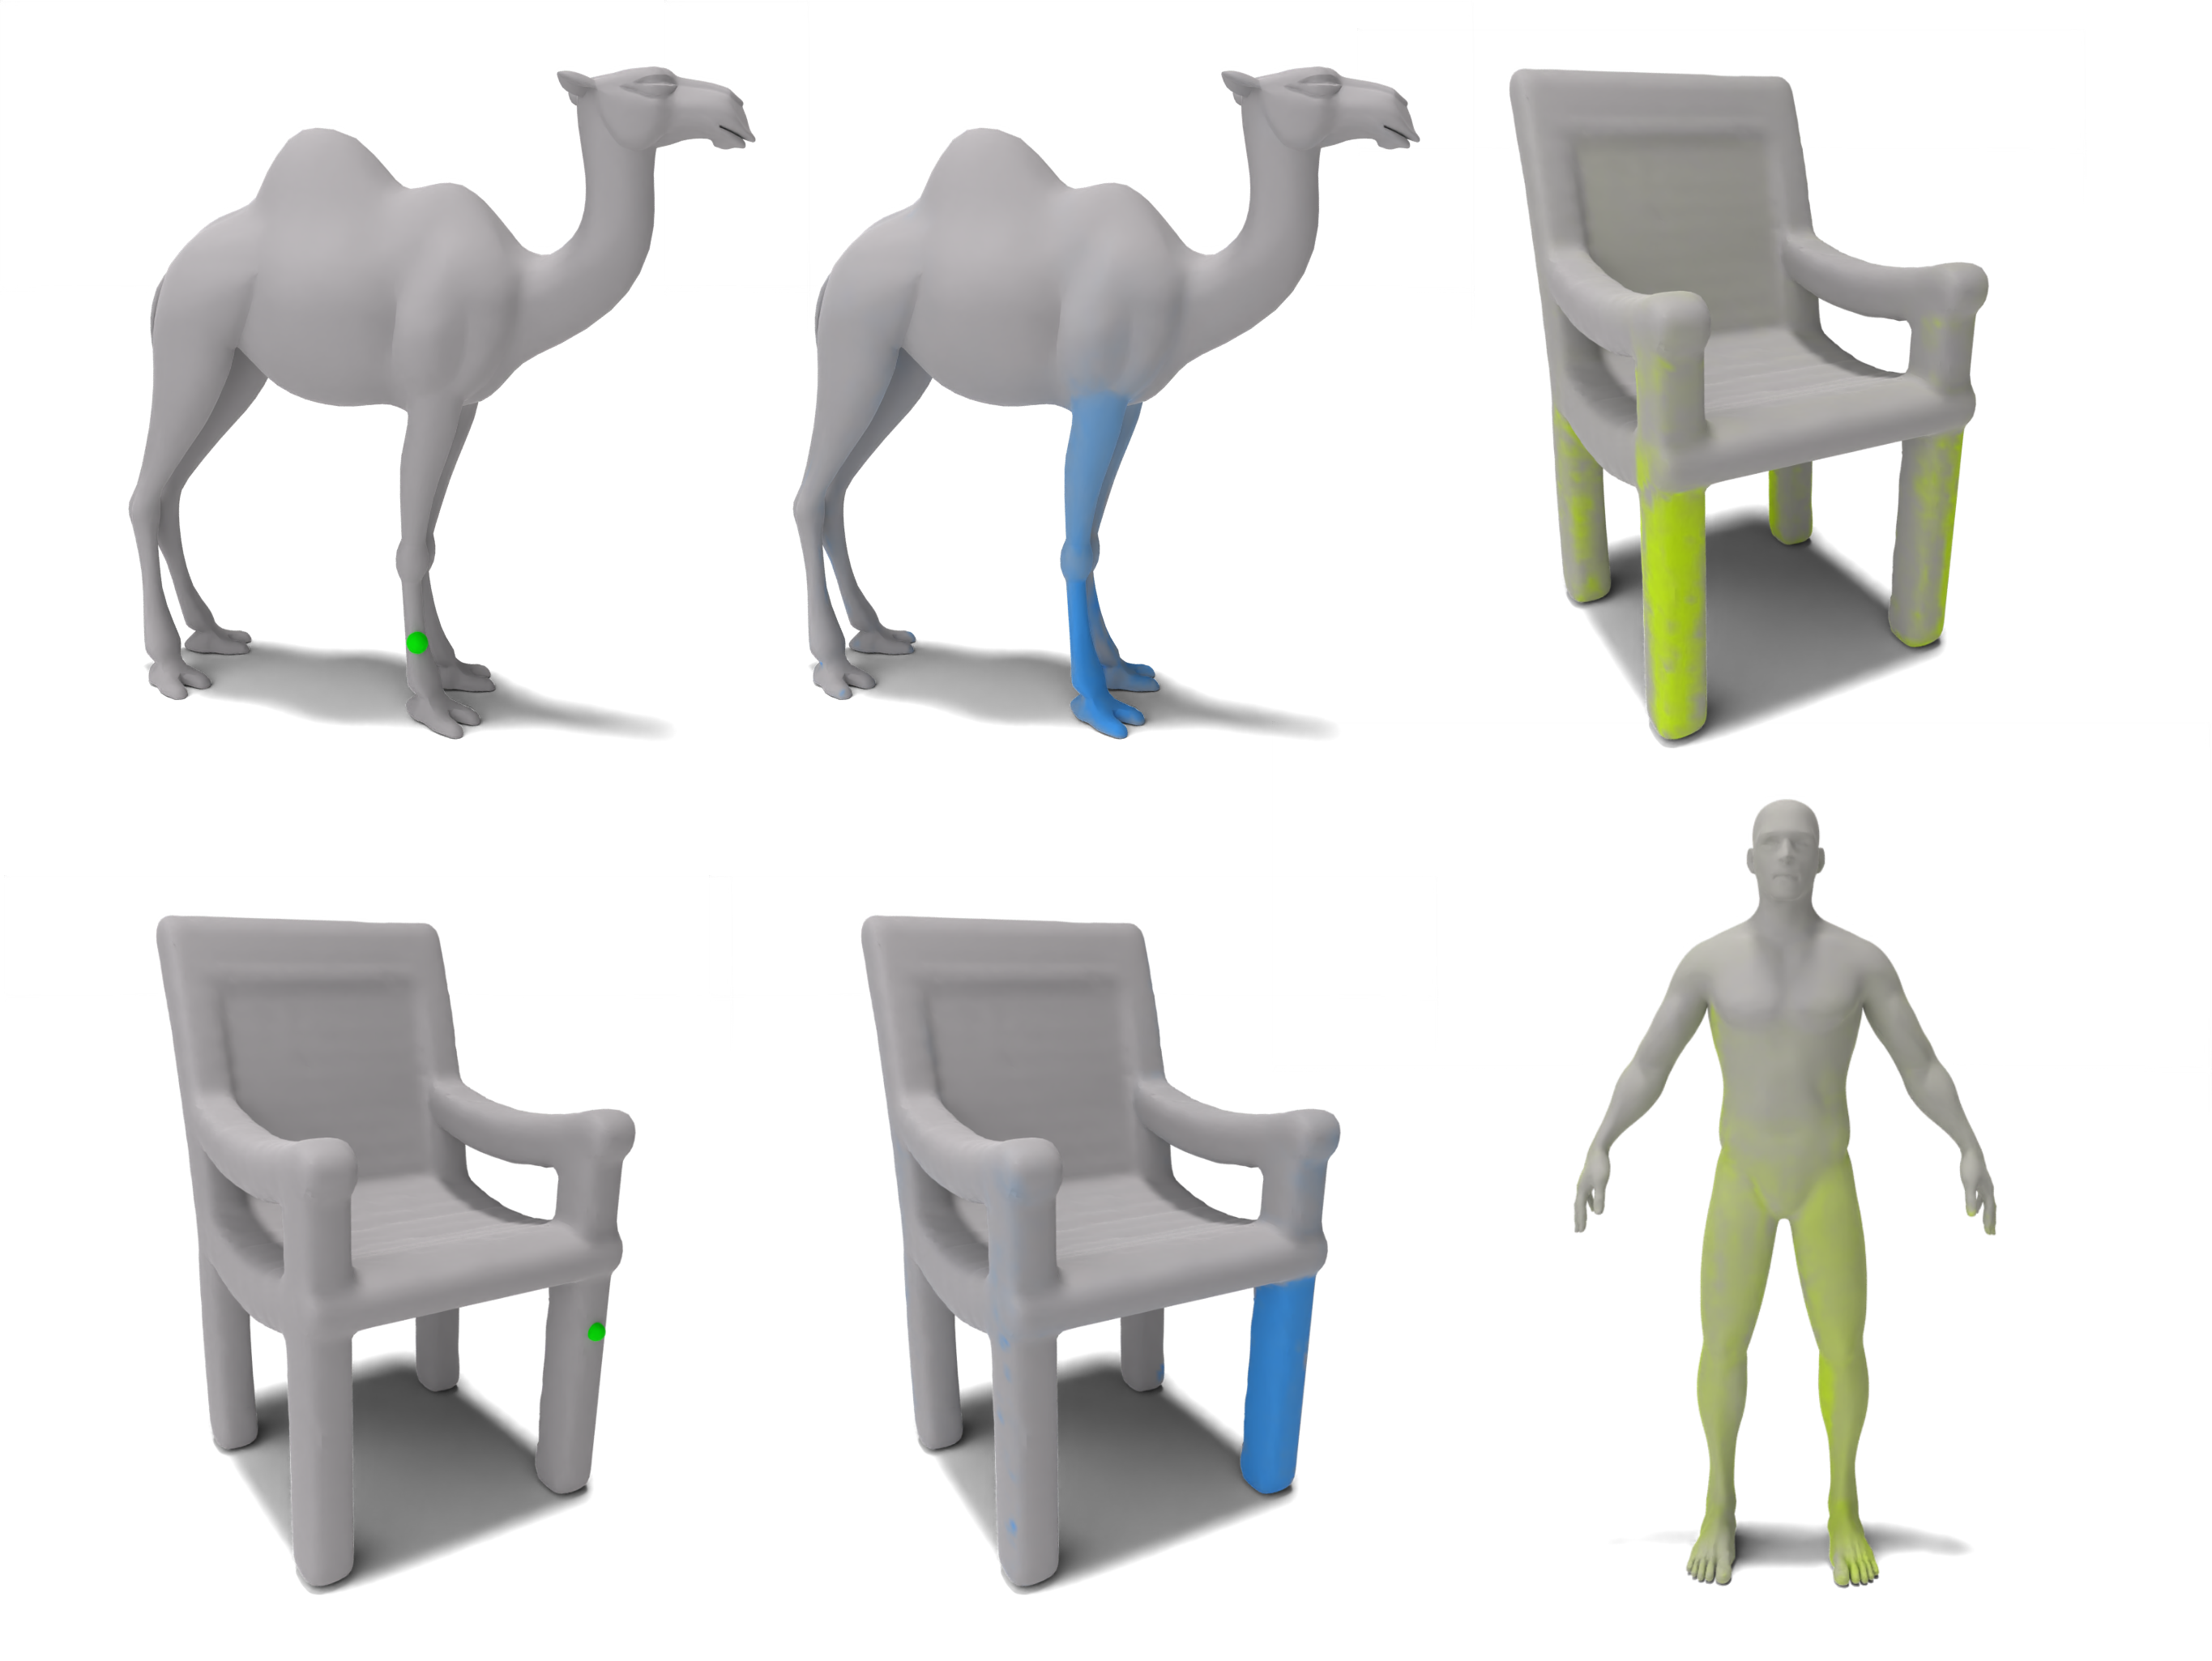}
\put(6,  \pl){\textcolor{black}{\small{Clicked point}}}
\put(38,  \pl){\textcolor{black}{\small{Self-segmentation}}}
\put(70,  \pl){\textcolor{black}{\small{Cross-segmentation}}}
\end{overpic}
\vspace{-2mm}
\captionof{figure}{\textbf{Cross-domain segmentation.} \ourmethod{} learned features generalize across domains. The feature vector of a clicked point results in the selection of a similar semantic region for the shape itself and a shape from a different domain.}
\label{fig:cross_supp}
\end{figure}
